# Supplementary material for: Uncoupled Learning Dynamics with $O(\log T)$ Swap Regret in Multiplayer Games
Source: arXiv:2204.11417 source file (2022-10-05)
Supplement: Supplementary file 1 [file appendix_bandit.tex]

\section{Proofs from \texorpdfstring{\Cref{section:bandit}}{Section 4}}
\label{appendix:bandit}

In this section we provide all the omitted proofs from \Cref{section:bandit}. Let us first introduce some further notation. We let $\last^{(t)}[a]$ be the recent time action $a$ was played prior to time $t$; that is, $\last^{(t)}[a] \defeq \max \{ \tau < t : a^{(\tau)} = a \}$, or $0$ if that set is empty. Further, for a \io{strictly?} convex function $\cR$ we let $D_{\cR}(\Vec{x}, \tilx) \defeq \cR(\Vec{x}) - \cR(\tilx) - \langle \nabla \cR(\tilx), \Vec{x} - \tilx \rangle$ be the \emph{Bregman divergence} induced by $\cR$. In this context, \emph{optimistic mirror descent (OMD)}~\citep{Rakhlin13:Optimization} in the bandit setting is parameterized by a prediction vector $\Vec{m}^{(t)}$ and an unbiased estimator $\hatu^{(t)}$ of $\Vec{u}^{(t)}$, and takes the following form for $t \in \N$:
\begin{equation}
    \label{eq:OMD}
    \tag{OMD}
    \begin{split}
        \Vec{x}^{(t+1)} &\defeq \argmax_{\Vec{x} \in \cX} \left\{ \eta \langle \Vec{x}, \Vec{m}^{(t+1)} \rangle - D_{\cR}(\Vec{x}, \Vec{g}^{(t)}) \right\}; \\
        \Vec{g}^{(t+1)} &\defeq \argmax_{\Vec{g} \in \cX} \left\{ \eta \langle \Vec{g}, \hatu^{(t+1)} \rangle - D_{\cR}(\Vec{g}, \Vec{g}^{(t)}) \right\}.
    \end{split}
\end{equation}
Further, we initialize with $\Vec{g}^{(1)} \defeq \argmin_{\Vec{g} \in \cX} \cR(\Vec{g})$. In the sequel, we focus on the MAB setting wherein $\cR$ is the log-barrier regularizer. We will use the following guarantee~\citep[Corollary 9]{Wei18:More}, where by convention we assume that $\Vec{u}^{(0)} \defeq \vec{0}$.

\begin{proposition}[\citep{Wei18:More}]
    \label{proposition:OMD-bandit}
    \eqref{eq:OMD} with prediction $\Vec{m}^{(t)}[a] \defeq \Vec{u}^{\last^{(t)}[a]}[a]$, estimated utility $\hatu^{(t)}[a] \defeq \frac{(\Vec{u}^{(t)}[a] - \Vec{m}^{(t)}[a]) \mathbbm{1}\{a^{(t)} = a \} }{\Vec{x}^{(t)}[a]} + \Vec{m}^{(t)}[a]$, for all $a \in \cA$, and $\eta \leq \frac{1}{162}$ satisfies
    \io{Be careful about the comparator}
    \begin{equation*}
        \E[\reg^T] \leq \frac{|\cA| \log T}{\eta} + \E\left[ 6 \eta \sum_{t=1}^T \| \Vec{u}^{(t)} - \Vec{u}^{(t-1)} \|_1 - \frac{1}{48\eta} \sum_{t=2}^T \|\Vec{x}^{(t)} - \Vec{x}^{(t-1)} \|^2_{\Vec{x}^{(t-1)}} \right].
    \end{equation*}
\end{proposition}

The following stability guarantee follows similarly to \Cref{lemma:stability}.

\begin{lemma}[Stability of OMD]
    \label{lemma:stab-OMD}
Let $\eta > 0$ be such that $\eta \| \hatu^{(t)} - \Vec{m}^{(t)}\|_{*, \Vec{x}^{(t)}} \leq \frac{1}{2}$ and $\eta \| \vec{m}^{(t)} \|_{*, \vec{g}^{(t-1)}} \leq \frac{1}{2}$. Then, for $t \in \N$,
\begin{equation*}
    \begin{split}
    \| \Vec{x}^{(t)} - \Vec{g}^{(t)} \|_{\Vec{x}^{(t)}} \leq 2 \eta \| \hatu^{(t)} - \Vec{m}^{(t)}\|_{*, \Vec{x}^{(t)}}; \\
    \| \Vec{x}^{(t)} - \Vec{g}^{(t-1)} \|_{\Vec{g}^{(t-1)}} \leq 2 \eta \| \Vec{m}^{(t)} \|_{*, \Vec{g}^{(t-1)}}.
    \end{split}
\end{equation*}
\end{lemma}
\begin{proof}
Let 
\begin{equation*}
    \begin{split}
        \Phi^{(t)}(\Vec{x}) \defeq \eta \langle \Vec{x}, \Vec{m}^{(t)} \rangle - \cR(\Vec{x}) + \langle \Vec{x}, \nabla \cR(\Vec{g}^{(t-1)}) \rangle; \\
        \Psi^{(t)}(\Vec{g}) \defeq \eta \langle \Vec{g}, \hatu^{(t)} \rangle - \cR(\Vec{g}) + \langle \Vec{g},  \nabla \cR(\Vec{g}^{(t-1)}) \rangle.
    \end{split}
\end{equation*}
Thus, it follows that $\nabla \Phi^{(t)}(\Vec{g}^{(t-1)}) = \eta \Vec{m}^{(t)}$, in turn implying that $\| \nabla \Phi^{(t)}(\Vec{g}^{(t-1)}) \|_{*, \Vec{g}^{(t-1)}} = \eta \| \Vec{m}^{(t)} \|_{*, \Vec{g}^{(t-1)}} \leq \frac{1}{2}$, by assumption. As a result, applying \Cref{lemma:stability-lam} yields that 
\begin{equation*}
    \| \Vec{x}^{(t)} - \Vec{g}^{(t-1)} \|_{\Vec{g}^{(t-1)}} = \| \Vec{g}^{(t-1)} - \argmin (- \Phi^{(t)}) \|_{\Vec{g}^{(t-1)}} \leq 2 \| \nabla \Phi^{(t)} (\Vec{g}^{(t-1)}) \|_{*, \Vec{g}^{(t-1)}} = 2\eta \| \Vec{m}^{(t)} \|_{*, \Vec{g}^{(t-1)}}.
\end{equation*}
Similarly, by the first-order optimality condition we have that $ \nabla \Phi^{(t)}(\Vec{x}^{(t)}) = \Vec{0} \iff \nabla \cR(\Vec{x}^{(t)}) = \nabla \cR(\Vec{g}^{(t-1)}) + \eta \vec{m}^{(t)}$. Thus, $\nabla \Psi(\Vec{x}^{(t)}) = - \nabla \cR(\Vec{x}^{(t)}) + \nabla \cR(\Vec{g}^{(t-1)}) + \eta \hatu^{(t)} = \eta (\hatu^{(t)} - \vec{m}^{(t)}) \leq \frac{1}{2}$, by assumption. As a result,
\begin{equation*}
    \| \Vec{x}^{(t)} - \Vec{g}^{(t)} \|_{\Vec{x}^{(t)}} = \| \Vec{x}^{(t)} - \argmin (- \Psi^{(t)}) \|_{\Vec{x}^{(t)}} \leq 2 \| \nabla \Psi^{(t)} (\Vec{x}^{(t)}) \|_{*, \Vec{x}^{(t)}} = 2 \eta \| \Vec{m}^{(t)} \|_{*, \Vec{x}^{(t)}}.
\end{equation*}
\end{proof}

\begin{corollary}[Multiplicative Stability]
    Let $\eta \in (0, \frac{1}{4}]$ be such that $\eta \|\hatu^{(t)} - \vec{m}^{(t)} \|_{*, \vec{x}^{(t)}} \leq \frac{1}{2}$ and $\eta \| \vec{m}^{(t)} \|_{*, \vec{g}^{(t-1)}} \leq \frac{1}{2}$. Then, for $t \geq 2$,
    \begin{equation*}
        \| \vec{x}^{(t)} - \vec{x}^{(t-1)} \|_{\vec{x}^{(t-1)}} \leq 4 \eta \| \vec{m}^{(t)} \|_{*, \vec{g}^{(t-1)}} + 2 \eta \|\hatu^{(t-1)} - \vec{m}^{(t-1)} \|_{*, \vec{x}^{(t-1)}}.
    \end{equation*}
\end{corollary}

\begin{proof}
Now applying the triangle inequality yields that $\| \vec{x}^{(t)} - \vec{x}^{(t-1)} \|_{\vec{x}^{(t-1)}} \leq \| \vec{x}^{(t)} - \vec{g}^{(t-1)} \|_{\vec{x}^{(t-1)}} + \| \vec{g}^{(t-1)} - \vec{x}^{(t-1)} \|_{\vec{x}^{(t-1)}}$. Since $\| \vec{x}^{(t)} - \vec{g}^{(t)} \|_{\vec{x}^{(t)}} \leq 2 \eta$, by assumption, it follows that $\| \vec{x}^{(t)} - \vec{g}^{(t-1)} \|_{\vec{x}^{(t-1)}} \leq 2 \| \vec{x}^{(t)} - \vec{g}^{(t-1)} \|_{\vec{g}^{(t-1)}}$ (for $\eta \leq \frac{1}{4}$). Thus,
\begin{align*}
\| \vec{x}^{(t)} - \vec{x}^{(t-1)} \|_{\vec{x}^{(t-1)}} &\leq 2 \| \vec{x}^{(t)} - \vec{g}^{(t-1)} \|_{\vec{g}^{(t-1)}} + \| \vec{g}^{(t-1)} - \vec{x}^{(t-1)} \|_{\vec{x}^{(t-1)}} \\
    &\leq 4 \eta \| \vec{m}^{(t)} \|_{*, \vec{g}^{(t-1)}} + 2 \eta \|\hatu^{(t-1)} - \vec{m}^{(t-1)} \|_{*, \vec{x}^{(t-1)}},
\end{align*}
by \Cref{lemma:stab-OMD}.
\end{proof}

Now from \Cref{proposition:OMD-bandit}, we get that the expected regret of each individual regret minimizer is such that
\begin{equation}
    \label{eq:rega-exp}
        \E[\reg_a^T] \leq \frac{|\cA| \log T}{\eta} + \E\left[ 6 \eta \sum_{t=1}^T \| \Vec{u}_a^{(t)} - \Vec{u}_a^{(t-1)} \|_1 - \frac{1}{48\eta} \sum_{t=2}^T \|\Vec{x}_a^{(t)} - \Vec{x}_a^{(t-1)} \|^2_{\Vec{x}_a^{(t-1)}} \right],
\end{equation}
for all $a \in \cA$, where recall that $\vec{u}_a^{(t)} = \vec{x}^{(t)}[a] \vec{u}^{(t)}$.
