# Supplementary material for: Uncoupled Learning Dynamics with $O(\log T)$ Swap Regret in Multiplayer Games
Source: arXiv:2204.11417 source file (2022-10-05)
Supplement: Supplementary file 2 [file appendix_phi.tex]

\section{Extension to General Phi-Regret Learners}
\label{sec:phi}

Suppose that $\cX \subseteq [0, 1]^d$ is a nonempty convex and compact set. \io{we may also need that $\Vec{0} \notin \cX$}---to make the rational function below well-defined. Further, let $\Phi \ni \phi : \cX \to \cX$ be a set of functions. \io{$\phi$ should include the identity mapping} Every function $\phi$ is uniquely represented by a vector $\vX \subseteq [0,1]^{\phidim} $. We will make the following assumption.

\begin{assumption}
    \label{assumption:rational}
For any function $\phi \in \Phi$ the following properties hold.
\begin{itemize}
    \item There exists $\vxstar \in \cX$ such that $\phi(\vxstar) = \vxstar$; and \io{we also need something along the lines: for any $\vX$ in the relative interior this fixed point is unique??}
    \item if $\phi$ is represented by $\vX \in [0,1]^D$, then for any $\ind \in \range{d}$,
    \begin{equation}
        \vxstar (\ind) = \sum_{k=1}^m \frac{p_{r, k}(\vX)}{q_{r, k}(\vX)},
    \end{equation}
    for some multivariate polynomials $p_{\cdot, \cdot}, q_{\cdot, \cdot} : \vX \mapsto \R$. We will further assume that $p_{\cdot, \cdot}(\Vec{0}), q_{\cdot, \cdot}(\Vec{0}) = 0$.
\end{itemize}
\end{assumption}

\begin{proposition}
    Assuming that all the polynomials in \Cref{assumption:rational} have positive coefficients is generic---under some assumptions on $\vX$.
\end{proposition}

\begin{proposition}[RVU for $\vX$ space]
    Direct from~\citep{Farina22:Near}.
\end{proposition}

\begin{proposition}
    Efficient implementation of the log-barrier on the $\vX$ space: show that the proximal oracle can be efficiently implemented.
\end{proposition}

\begin{proof}
    \io{If we can implement the oracle for each set, can we do it for its convex hull?}
\end{proof}

\begin{lemma}
Suppose that $\Phi$ satisfies \Cref{assumption:rational}. If the learning rate is sufficiently small $\eta = O(\frac{1}{\deg})$, then for any $t \in \N$,
\begin{equation*}
    \| \vx^{(t)} - \vx^{(t-1)} \|_1^2 \leq 36 \|\cX\|_1^2 \deg^2 \|\vX^{(t)} - \vX^{(t-1)} \|^2_{\vX^{(t-1)}}.
\end{equation*}
\end{lemma}

The proof of this lemma is similar to~\Cref{lemma:gamma-term}, but we include it for completeness.

\begin{proof}
    Fix any $t \in \N$, and let us define
    \begin{equation}
        \label{eq:defmul}
        \mul^{(t)} \defeq \max_{\edg \in \range{D}} \left| 1 - \frac{\vX^{(t)}[\edg]}{\vX^{(t-1)}[\edg]} \right|,
    \end{equation}
    for $t \in \N$. Further, in the context of \Cref{assumption:rational}, suppose that
    \begin{equation}
        p_{\ind,k} : \vX \mapsto \sum_{\tree \in \treeset_{\ind, k}} C_{\tree} \prod_{\edg \in \tree} \vX[\edg],
    \end{equation}
    and
    \begin{equation}
        q_{\ind, k}: \vX \mapsto \sum_{\tree \in \treeset'_{\ind, k}} C_{\tree} \prod_{\edg \in \tree} \vX[\edg],
    \end{equation}
    for all $(\ind, k) \in \range{d} \times \range{m}$, where $C_{\tree} > 0$ for any $\tree \in \treeset_{\ind, k}$ and $C_{\tree} > 0$ for any $\tree \in \treeset'_{\ind, k}$.
    Then, for $(r,k) \in \range{d} \times \range{m}$,
    \begin{align}
        p_{\ind, k}(\vX^{(t)}) &= \sum_{\tree \in \treeset_{\ind, k}} C_{\tree} \prod_{\edg \in \tree} \vX^{(t)}[\edg] \notag \\
        &\leq \sum_{\tree \in \treeset} C_{\tree} \prod_{\edg \in \tree} (1 + \mul^{(t)}) \vX^{(t-1)}[\edg] \label{align:mulX} \\
        &\leq (1 + \mul^{(t)})^{\deg} \sum_{\tree \in \treeset_{\ind, k}} C_{\tree} \prod_{\edg \in \tree} \vX^{(t-1)}[\edg] \label{align:deg} \\
        &= (1 + \mul^{(t)})^{\deg} p_{\ind, k}(\vX^{(t-1)}) \notag \\
        &\leq (1 + 2 \mul^{(t)} \deg) p_{\ind, k}(\vX^{(t-1)}), \label{align:calc}
    \end{align}
    where \eqref{align:mulX} follows since $\vX^{(t)}[\edg] \leq (1 + \mul^{(t)}) \vX^{(t-1)}[\edg]$, for any $\edg \in \range{D}$, by definition of $\mul^{(t)}$ in \eqref{eq:defmul}; \eqref{align:deg} uses the fact that $|\tree| \leq \deg$ for any $\tree \in \treeset_{\ind, k}$; and \eqref{align:calc} follows since $(1 + \mul^{(t)})^{\deg} \leq \exp \{ \mul^{(t)} \deg \} \leq 1 + 2 \mul^{(t)} \deg$ for $\mul^{(t)} \leq \frac{1}{\deg}$. Similarly, for $(\ind, k) \in \range{d} \times \range{m}$, we get
    \begin{align}
        p_{\ind, k}(\vX^{(t)}) &= \sum_{\tree \in \treeset_{\ind, k}} C_{\tree} \prod_{\edg \in \tree} \vX^{(t)}[\edg] \notag \\
        &\geq \sum_{\tree \in \treeset_{\ind, k}} C_{\tree} \prod_{\edg \in \tree} (1 - \mul^{(t)}) \vX^{(t-1)}[\edg] \notag \\
        &\geq (1 - \mul^{(t)})^{\deg} p_{\ind, k}(\vX^{(t-1)}) \notag \\
        &\geq (1 - \mul^{(t)} \deg) p_{\ind, k}(\vX^{(t-1)}),\label{align:finalp}
    \end{align}
    where the last bound follows from Bernoulli's inequality. Analogous reasoning yields that for any $(\ind, k) \in \range{d} \times \range{m}$,
    \begin{equation}
        \label{eq:q1}
        q_{\ind, k}(\vX^{(t)}) \leq (1 + 2 \mul^{(t)} \deg) q_{\ind, k}(\vX^{(t-1)}),
    \end{equation}
    and 
    \begin{equation}
        \label{eq:q2}
        q_{\ind, k}(\vX^{(t)}) \geq (1 - \mul^{(t)} \deg) q_{\ind, k}(\vX^{(t-1)}).
    \end{equation}
    As a result, for $\ind \in \range{d}$,
    \begin{align}
        \vx^{(t)}[\ind] - \vx^{(t-1)}[\ind] &= \sum_{k=1}^m \frac{p_{\ind, k}(\vX^{(t)})}{q_{\ind, k}(\vX^{(t)})} - \sum_{k=1}^m \frac{p_{\ind, k}(\vX^{(t-1)})}{q_{\ind, k}(\vX^{(t-1)})} \notag \\
        &\leq \sum_{k=1}^m \left( \frac{1 + 2 \mul^{(t)} \deg}{1 - \mul^{(t)} \deg} \right) \frac{p_{\ind, k}(\vX^{(t-1)})}{q_{\ind, k}(\vX^{(t-1)})} - \sum_{k=1}^m \frac{p_{\ind, k}(\vX^{(t-1)})}{q_{\ind, k}(\vX^{(t-1)})} \label{align:updown} \\
        &\leq \left( 1 + \frac{3 \mul^{(t)}\deg}{1 - \mul^{(t)} \deg} \right) \sum_{k=1}^m \frac{p_{\ind, k}(\vX^{(t-1)})}{q_{\ind, k}(\vX^{(t-1)})} - \sum_{k=1}^m \frac{p_{\ind, k}(\vX^{(t-1)})}{q_{\ind, k}(\vX^{(t-1)})} \notag \\
        &= \frac{3 \mul^{(t)}\deg}{1 - \mul^{(t)} \deg} \vx^{(t-1)}[\ind] \leq 6 \mul^{(t)} \deg \vx^{(t-1)}[\ind]. \label{align:onedif}
    \end{align}
    where \eqref{align:updown} uses \eqref{align:calc} and \eqref{eq:q2}, and \eqref{align:onedif} follows from the fact that $\mul^{(t)} \leq \frac{1}{2\deg}$. Similarly, by \eqref{align:finalp} and \eqref{eq:q1},
    \begin{equation*}
        \vx^{(t-1)}[\ind] - \vx^{(t)}[\ind] = \sum_{k=1}^m \frac{p_{\ind, k}(\vX^{(t-1)})}{q_{\ind, k}(\vX^{(t-1)})} - \sum_{k=1}^m \frac{p_{\ind, k}(\vX^{(t)})}{q_{\ind, k}(\vX^{(t)})} \leq 6 \mul^{(t)} \deg \vx^{(t-1)}[\ind].
    \end{equation*}
    As a result, we conclude that
    \begin{align*}
        \| \vx^{(t)} - \vx^{(t-1)} \|^2_1 &\leq 36 \left( \mul^{(t)} \deg \sum_{\ind=1}^d \vx^{(t-1)}[\ind] \right)^2 \leq 36 \|\cX\|^2_1 \deg^2 \max_{\edg \in \range{D}} \left( 1 - \frac{\vX^{(t)}[\edg]}{\vX^{(t-1)}[\edg]} \right)^2. \\
        &\leq 36 \|\cX\|_1^2 \deg^2 \|\vX^{(t)} - \vX^{(t-1)} \|^2_{\vX^{(t-1)}}.
    \end{align*}
    
\end{proof}
